# Supplementary material for: Logit Lens Supervision for Patch-Level Explanations in Vision-Language Models
Source: arXiv:2602.01530 source file (2026-08-11)
Supplement: Supplementary file 1 [file appendix.tex]

\subsection{Implementation Configuration}


We finetuned the LLava-v1.5-7B and Qwen2.5-VL-7B-Instruct VLMs using DeepSpeed on four NVIDIA A100 GPUs (80 GB VRAM each). The vision encoder remained frozen except for a trainable projection layer, while Low-Rank Adaptation (LoRA) was applied to the layers of the language model: both LLava-v1.5 and Qwen2.5-VL employed a LoRA rank of 16. Note that for the LLL(Logit Lens Loss), the language head, which represents the unembedding matrix, was frozen to stay consistent. Training was conducted with a per-GPU batch size of 16 and gradient accumulation of 4 (effective global batch size = 256). Optimization followed a cosine decay learning rate schedule (initial LR = $5\times10^{-5}$) with a linear warm-up over the first 3\% of total training steps. 
For all tasks except for the zero-shot pointing to objects, we finetuned the models for 1 epoch on the corresponding training sets.


For the commercial VLM baselines (GPT-4o and Gemini-2.0 Flash), we queried the public APIs using their default system prompts. We performed greedy decoding, did not apply top-$k$ or top-$p$ sampling, and left the temperature parameter at its default setting, ensuring that outputs were deterministic and directly comparable to those from our finetuned open-source models.


\paragraph{Training Prompt.}
We use the same prompt template for training and evaluation, instructing the VLM to output a single bounding box for the referred object:
\begin{quote}\small
\texttt{Given the image and the referring expression, output the bounding box coordinates of the referred object in pixel coordinates.}
\end{quote}


\paragraph{Logit Lens Confidence Map-to-Mask Generation and Thresholding.}
For heatmap thresholding, we binarize the heatmap using a scalar threshold $\tau$ computed from \textbf{per-image} heatmap statistics. We evaluate
\[
\tau \in \{\mu-\sigma,\ \mu,\ \mu+\sigma,\ \mathbb{E}[H]\},
\]
where $\mu$ and $\sigma$ are the mean and standard deviation of heatmap values for the given image, and $\mathbb{E}[H]$ denotes the mean of all values in the map of that image. Pixels with values above $\tau$ are retained in the binary mask. For Logit Lens maps, $\tau=\mu$ performs best.
\subsubsection{Ablations}
We first illustrate how the layer choice for applying the Logit Lens Loss (LLL) affects performance. As shown in
Table~\ref{tab:ablation_layers}, applying LLL to the \emph{last layer only}
achieves the best accuracy (93.87\%), outperforming the top-layer aggregation and
middle-layer aggregation. This is expected, as the final layer is most closely
aligned with the language head (unembedding matrix), making the LLL constraint
more effective.

Furthermore, Table~\ref{tab:lambda_ablation} the influence of the weighting
coefficient~$\lambda$ on the performance.
A moderate weighting provides
the strongest gains: accuracy peaks at $\lambda = 0.50$, while both smaller and larger values lead to slight declines. 

\begin{table}[!htbp]
  \centering
  \small
  \caption{Ablation of layer choices for Logit Lens loss on POPE dataset for \textit{Qwen2.5-VL-7B-Instr.} with \textbf{NTP + LLL}.}
  \label{tab:ablation_layers}
  \begin{tabular}{lc}
    \toprule
    \textbf{Layer} & \textbf{Accuracy (\%)} \\
    \midrule
    Top 4 Layers            & 90.86\% \\
    Middle layers (13--16)  & 91.37\% \\
    Last layer only         & \textbf{93.87}\% \\
    \bottomrule
  \end{tabular}
\end{table}

\begin{table}[!htbp]
  \centering
  \small
  \caption{Effect of varying the hyperparameter $\lambda$ in the combined loss 
  ($\mathcal{L}_{\text{total}} = \mathcal{L}_{\text{NTP}} + \lambda \mathcal{L}_{\text{LLL}}$) 
  on POPE for \textit{Qwen2.5-VL-7B-Instr.}}
  \label{tab:lambda_ablation}
  \begin{tabular}{lc}
    \toprule
    \textbf{$\lambda$} & \textbf{Accuracy (\%)} \\
    \midrule
    0.25 & 92.41\% \\
    0.50 & \textbf{93.87}\% \\
    0.75 & 93.12\% \\
    1.00 & 92.78\% \\
    \bottomrule
  \end{tabular}
\end{table}




\section{Complementary Localization Results}

We evaluate localization quality on the RefCOCO validation set, using models trained on the corresponding RefCOCO training split. To quantify how well visual tokens encode object-specific semantics after fine-tuning, we use two complementary metrics, both derived from the same per-patch
confidence values. The \emph{Object Confidence Ratio} (OCR), introduced in the
main paper, compares the average per-patch confidence inside the ground-truth
bounding box to the average over the whole image. The \emph{Energy Inside
Ground Truth} (EIGT) measures the fraction of the total activation (summed over
patches) that lies inside the bounding box. Together, these metrics quantify
how accurately and how strongly the model localizes the queried object.


\textbf{Object Confidence Ratio.} We use the same
per-patch confidence formulation introduced in Fig. 3.
Recall that each visual token $s$ in the last decoder layer produces a
probability
\[
CS_{\mathrm{patch}}(v,s)
= p_\theta\!\left(v \mid h_L(s)\right),
\]
where $v$ is a vocabulary token representing the queried object.
A region-level score $CS_{\mathrm{region}}(v,\mathcal{P}')$ is obtained by
averaging $CS_{\mathrm{patch}}$ over the visual tokens
$\mathcal{P}'$ covering the region (e.g., the bounding box).
The Object Confidence Ratio (OCR) used in the main paper compares how strongly the
model activates on the ground-truth region relative to the whole image:
\[
\mathrm{OCR}
= \frac{CS_{\mathrm{BB}}(v)}
        {CS_{\mathrm{image}}(v)}.
\]

\textbf{Energy Inside Ground Truth.} 
Let $h_L(x,y)\in\mathbb{R}^d$ denote the hidden state of the visual token at
spatial position $(x,y)$ in the last decoder layer. Using the model's 
unembedding matrix $U_\theta\in\mathbb{R}^{|\mathcal{V}|\times d}$, we obtain
vocabulary logits
\[
z(x,y) = U_\theta\, h_L(x,y) \in \mathbb{R}^{|\mathcal{V}|}.
\]
Let $\mathcal{V}_{\text{obj}} \subset \mathcal{V}$ be the set of vocabulary
tokens encoding the name of the queried object (e.g.\ \texttt{<dog>}, \texttt{<dining table>}, etc). The querried object could be comprised of multiple tokens. The object activation map is defined as
\[
H(x,y) = \max_{v \in \mathcal{V}_{\text{obj}}} z_v(x,y).
\]
Thus, $H$ measures how strongly the model associates each visual token with the
querried object.

Given a ground-truth bounding box $\mathrm{GT}$, we quantify localization via
the fraction of activation mass that lies inside the object region:
\[
\mathrm{EIGT}
=
\frac{\sum_{(x,y)\in\mathrm{GT}} H(x,y)}
     {\sum_{(x,y)} H(x,y)}.
\]
This threshold-free measure is equivalent to energy- and relevance-mass metrics
used in prior grounding work\cite{xiao2024towards}.


\begin{table}[h]
\centering
\setlength{\tabcolsep}{3pt} % decrease column spacing

\begin{tabular}{lcc}
\toprule
\textbf{Model} & \textbf{EIGT} & \textbf{OCR}  \\
\midrule
Qwen-2.5-VL      & 0.4278 & 3.7  \\
NTP               & 0.4763 & 3.5 \\
NTP + LLL         & \textbf{0.6657} & \textbf{9.9} \\
\bottomrule
\end{tabular}
\caption{Localization performance on the RefCOCO validation set for \textit{Qwen2.5-VL-7B-Instr.}}
\label{tab:localization_refcoco}
\end{table}

Table~\ref{tab:localization_refcoco} reports EIGT scores on the RefCOCO
validation set. The trend mirrors the Object Confidence Ratio (OCR) analysis
presented in the main paper: models finetuned with LLL allocate substantially
more activation mass to the correct spatial region. Taken together, the EIGT
and OCR results consistently show that LLL enhances the spatial grounding of
visual tokens and produces more localized, object-specific confidence maps.



%%%%%%%%%%%%%%%%%%%%%%%%%%
\begin{figure*}[!htbp]
  \centering
  % -------- Row 1 --------
   \begin{subfigure}[b]{0.24\textwidth}
    \includegraphics[width=\textwidth]{figures/supp/person.png}
    \caption{Object: Person}
  \end{subfigure}
  \begin{subfigure}[b]{0.24\textwidth}
    \includegraphics[width=\textwidth]{figures/supp/qwen_person_0.0006.png}
    \caption{CS = 0.0006}
  \end{subfigure}
  \hfill
  \begin{subfigure}[b]{0.24\textwidth}
    \includegraphics[width=\textwidth]{figures/supp/ntp_person_0.001.png}
    \caption{CS = 0.001}
  \end{subfigure}
  \hfill
  \begin{subfigure}[b]{0.24\textwidth}
    \includegraphics[width=\textwidth]{figures/supp/lll_person_0.04.png}
    \caption{CS = 0.04 }
  \end{subfigure}
  % \vspace{1em}
  \caption{An example of Object confidence maps not being able to perfectly localize the objects within the image for object "person" with multiple instances taking a lot of space. First column: actual image with the text token for localization, second: base model, third: NTP finetuned, fourth: NTP+LLL finetuned. The numbers indicate the BB confidence score $CS_{BB}$ for the target objects, i.e., the average confidence that a given object is present in the patches in the ground truth BB.
  }
  \label{fig:confidence_maps}
\end{figure*}





\subsection{Layer‐wise Visual Attention}
Fig.~\ref{fig:layerwise-attention} compares the per‐layer sum of attention weights to visual tokens for the LLava‐v1.5 and Qwen2.5‐VL base models. Across layers, the attention of the last answer token to visual tokens comprises about 10.93\%(SD ± 12.66\%) of the total attention to all tokens in LLava-v1.5, which is substantially higher than Qwen-2.5VL’s average of 2.33\% (SD ± 1.44\%). We evaluated both models on Pope dataset.

\begin{figure}[!htbp]
  \centering
  \begin{subfigure}[b]{0.48\textwidth}
    \includegraphics[width=\textwidth]{figures/supp/llava_attention_individual.png}
    \caption{LLava-v1.5-7B Base Model}
    \label{fig:attention-llava}
  \end{subfigure}
  \quad
  \begin{subfigure}[b]{0.48\textwidth}
    \includegraphics[width=\textwidth]{figures/supp/qwen_attention_individual.png}
    \caption{Qwen2.5-VL-7B-Instruct Base Model}
    \label{fig:attention-qwen}
  \end{subfigure}
  \caption{Layer-wise visual attention analysis (sum of attention weights to visual tokens) for LLava-v1.5 and Qwen-2.5VL.}
  \label{fig:layerwise-attention}
\end{figure}









\begin{table}[!t]
  \centering

  \caption{Comparison on the REC (Referring Expression Comprehension) task measured by IoU@0.5. SOTAs are finetuning based VLMs.}
  \label{tab:refcoco_dataset_performance}
  % \setlength{\tabcolsep}{6pt}
  % \begin{tabular}{lccc}
  {\small
    \setlength{\tabcolsep}{2pt} % tighter columns (default ≈ 6pt)

    \begin{tabular}{l@{\hspace{0pt}}ccc}

    \toprule
    % \textbf{Method} & \textbf{RefCOCO} & \textbf{RefCOCO+}& \textbf{RefCOCOg} \\
\textbf{Method} & {\scriptsize\textbf{RefCOCO}} & {\scriptsize\textbf{RefCOCO+}} & {\scriptsize\textbf{RefCOCOg}} \\


    \midrule
    \multicolumn{4}{l}{\textit{LLaVA-v1.5-7B}} \\
    \quad Base Model & 52.90 & 42.55 & 45.00 \\
    \quad NTP & 53.20 & 42.90 & 45.40 \\
    \quad NTP + LLL & 53.95 & 43.40 & 46.00 \\
    \midrule
    \multicolumn{4}{l}{\textit{Qwen2.5-VL-7B-Instr.}} \\
    \quad Base Model & 90.05 & 85.40 & 86.60 \\
    \quad NTP & 90.60 & 85.70 & 86.80 \\
    % \quad NTP + LLL & 91.50 & 86.40 &  87.30 \\
 \quad NTP + LLL & \second{91.50} & \second{86.40} & \second{87.30} \\

    \midrule
    \multicolumn{4}{l}{\textit{SOTA}} \\
    \quad LLaVA-G-7B \tcite{zhang2023llavagroundinggroundedvisualchat} & 89.16 & 81.68 & 84.82\\
    \quad Shikra-7B \tcite{chen2023shikraunleashingmultimodalllms} & 87.0 & 81.6 & 82.3 \\
    \quad Ferret-7B \tcite{you2023ferretrefergroundgranularity} & 87.5 & 80.8 & 83.9 \\
    \quad Shikra-13B \tcite{chen2023shikraunleashingmultimodalllms} & 87.8 & 82.9 & 82.6 \\
    \quad Ferret-13B \tcite{you2023ferretrefergroundgranularity} & 89.5 & 82.8 & 85.8 \\
    % \quad CogVLM-17B \tcite{wang2024cogvlmvisualexpertpretrained} & \textbf{92.8} & \textbf{88.7} & \textbf{89.8} \\
   \quad CogVLM-17B \tcite{wang2024cogvlmvisualexpertpretrained} 
& \best{92.8} & \best{88.7} & \best{89.8} \\

    \bottomrule
  \end{tabular}
  }
\end{table}



\section{Object Confidence Map Limitation}
Fig. ~\ref{fig:confidence_maps} shows a case where object confidence maps
struggle to localize targets when multiple instances of the same category (e.g.,
\textit{person}) occupy much of the image. 
The base model exhibits broad activations, NTP finetuning improves focus, and
NTP+LLL provides the most concentrated localization, though challenges remain in
crowded scenes with objects composed of a relatively large number of patches.



% You can have as much text here as you want. The main body must be at most $8$
% pages long. For the final version, one more page can be added. If you want, you
% can use an appendix like this one.

% The $\mathtt{\backslash onecolumn}$ command above can be kept in place if you
% prefer a one-column appendix, or can be removed if you prefer a two-column
% appendix.  Apart from this possible change, the style (font size, spacing,
% margins, page numbering, etc.) should be kept the same as the main body.
%%%%%%%%%%%%%%%%%%%%%%%%%%%%%%%%%%%%%%%%%%%%%%%%%%%%%%%%%%%%%%%%%%%%%%%%%%%%%%%
%%%%%%%%%%%%%%%%%%%%%%%%%%%%%%%%%%%%%%%%%%%%%%%%%%%%%%%%%%%%%%%%%%%%%%%%%%%%%%%




\textbf{Referring Expression Comprehension (REC).}
Table~\ref{tab:refcoco_dataset_performance} compares our approach with existing SOTA models on the RefCOCO, RefCOCO+, and RefCOCOg benchmarks. Finetuning with LLL consistently improves performance over both the base and NTP-finetuned models across all datasets. The Qwen2.5-VL model with LLL achieves results that rival or surpass several SOTA VLMs, while approaching the performance of substantially larger models like CogVLM with 17B parameters. These findings demonstrate that LLL provides competitive grounding capabilities without introducing architectural changes, highlighting its effectiveness as a lightweight yet powerful auxiliary objective for enhancing visual alignment in VLMs.
